# Supplementary material for: Online Control of the False Discovery Rate under "Decision Deadlines"
Source: arXiv:2110.01583 ancillary file (2021-10-15)
Supplement: Supplementary file 1 [file online_FDR_TOAD-decision-v11-aistats-supp.pdf]

# Supplementary Materials for *Online Control of the False Discovery Rate under "Decision Deadlines"*

Aaron Fisher*

October 15, 2021

## Brief note on cross-references

Throughout this supplement, we use letter prefixes when referring to items within the supplementary materials (e.g., Eq (B.1) in Section B of the supplement), and use regular numeric references for items in the main text (e.g., Eq (1) in Section 2 of the main text).

# A Proofs

## A.1 Proof of Monotonicity

In this section, we show that TOAD never reverses a previous rejection. This is formalized in the following lemma.

**Lemma A.1.** *(No rejection reversals) The rejection sets produced by TOAD satisfy $\mathcal{R}_t \subseteq \mathcal{R}_{t'}$ for any $0 < t < t' < \infty$.*

*Proof.* We will show the result by induction. We start by showing that any hypothesis index $j$ that is rejected at any stage $t$ remains rejected at stage $t+1$ (i.e., if $j \in \mathcal{R}_t$ then $j \in \mathcal{R}_{t+1}$).

Let $\mathcal{A}_t = \mathcal{R}_t \cap \mathcal{C}_t \cap \mathcal{C}_{t+1}$ be the subset of indices rejected at time $t$ that are active candidates at both stage $t$ and $t+1$. Let $\mathcal{N}_t = \{\mathcal{R}_t \cap \mathcal{C}_t\} \backslash \mathcal{C}_{t+1}$ be the subset of indices rejected at time $t$ that are active candidates at time $t$, but *not* at time $t+1$. Since $S_t = |\mathcal{C}_t \cap \mathcal{R}_t|$ is equal to the number of hypotheses that are both active and rejected at stage $t$, we have $S_t = |\mathcal{A}_t| + |\mathcal{N}_t|$.

Assume that $j \in \mathcal{R}_t$. If $j \notin \mathcal{C}_{t+1}$, then $j \in \mathcal{R}^{\text{old}}_{t+1}$, and the fact that $j \in \mathcal{R}_{t+1}$ holds automatically. Likewise if $j \notin \mathcal{C}_t$ then $j \notin \mathcal{C}_{t+1}$ (by definition) and the result again holds automatically. Otherwise, we must have $j \in \mathcal{A}_t$. So, hereafter, we assume that $j \in \mathcal{A}_t$.

We now consider two cases, depending on and whether or not adding $W_{t+1}$ in stage $t+1$ changes the ordering of the test statistics $\{W_i\}_{i \in \mathcal{A}_t}$.

**Case-1** $W_{t+1} \geq \max_{i \in \mathcal{A}_t} W_i$: Here, the test statistics $\{W_i\}_{i \in \mathcal{A}_t}$ advance to become the lowest $|\mathcal{A}_t|$ values in the new set of active statistics $\{W_i\}_{i \in \mathcal{C}_{t+1}}$, meaning that $W_{(|\mathcal{A}_t|, t+1)} = \max_{i \in \mathcal{A}_t} W_i$. Applying this, we have

$$\begin{aligned} W_{(|\mathcal{A}_t|,t+1)} = \max_{i \in \mathcal{A}_t} W_i \leq W_{(S_t,t)} \leq & \alpha\beta \left( S_t + |\mathcal{R}^{\text{old}}_t| \right) \\ = & \alpha\beta \left( |\mathcal{A}_t| + |\mathcal{N}_t| + |\mathcal{R}^{\text{old}}_t| \right) \\ = & \alpha\beta \left( |\mathcal{A}_t| + |\mathcal{R}^{\text{old}}_{t+1}| \right). \end{aligned} \tag{A.1}$$

Thus, from the definition of $S_{T+1}$ (Eq (3)) we have $|\mathcal{A}_t| \leq S_{T+1}$. Finally, since

$$W_j \leq \max_{i \in \mathcal{A}_t} W_i = W_{(|\mathcal{A}_t|,t+1)} \leq W_{(S_{T+1},t+1)},$$

*Foundation Medicine Inc.; 150 Second St, Cambridge, MA 02141. afishe27@alumni.jh.edu

we see that $j$ is rejected in stage $t+1$.

**Case-2** $W_{t+1} < \max_{i \in \mathcal{A}_t} W_i$: Here, the test statistics $\{W_i\}_{i \in \mathcal{A}_t} \cup W_{t+1}$ become the lowest $(|\mathcal{A}_t| + 1)$ values in the new set of active statistics $\{W_i\}_{i \in \mathcal{C}_{t+1}}$, and so $\max_{i \in \mathcal{A}_t} W_i = W_{(|\mathcal{A}_t|+1, t+1)}$. Following the same steps as above, we have

$$\begin{aligned}
W_{(|\mathcal{A}_t|+1,t+1)} = \max_{i \in \mathcal{A}_t} W_i \leq W_{(S_t,t)} &\leq \alpha\beta\left(S_t + |\mathcal{R}_t^{\text{old}}|\right) \\
&= \alpha\beta\left(|\mathcal{A}_t| + |\mathcal{N}_t| + |\mathcal{R}_t^{\text{old}}|\right) \\
&= \alpha\beta\left(|\mathcal{A}_t| + |\mathcal{R}_{t+1}^{\text{old}}|\right) \\
&\leq \alpha\beta\left(|\mathcal{A}_t| + 1 + |\mathcal{R}_{t+1}^{\text{old}}|\right),
\end{aligned}$$

where, in the last line, we use the fact that both shape functions and the identity function are nondecreasing. From the definition of $S_{T+1}$ we have $|\mathcal{A}_t| + 1 \leq S_{T+1}$. Finally, since

$$W_j \leq \max_{i \in \mathcal{A}_t} W_i = W_{(|\mathcal{A}_t|+1,t+1)} \leq W_{(S_{T+1},t+1)},$$

we see that $j$ is rejected in stage $t+1$.

Thus, for any $j \in \mathcal{R}_t$, we know that $j \in \mathcal{R}_{t+1}$. It now follows by induction that $j \in \mathcal{R}_{t'}$. □

## A.2 Proof of Theorem 1

### Part 1

*Proof.* Suppose the $H_i$ is rejected at stage $t$, and let $T_i \leq t$ be the *first* stage at which $H_i$ is rejected. We know that

$$W_i \leq W_{(S_{T_i},T_i)} \leq \alpha\beta\left(S_{T_i} + |\mathcal{R}_{T_i}^{\text{old}}|\right) = \alpha\beta\left(|\mathcal{R}_{T_i}|\right) \leq \alpha\beta\left(1 \vee |\mathcal{R}_{T_i}|\right).$$

From Lemma A.1, and from the fact that $\beta$ (the identity function) is nondecreasing, we have

$$W_i \leq \alpha\beta\left(1 \vee |\mathcal{R}_{T_i}|\right) \leq \alpha\beta\left(1 \vee |\mathcal{R}_t|\right). \tag{A.2}$$

Finally, plugging in $W_i = P_i/A_i$, we see that rejecting any hypothesis $H_i$ by time $t$ requires

$$\begin{aligned}
P_i/A_i &\leq \beta\left(1 \vee |\mathcal{R}_t|\right)\alpha \\
P_i &\leq \beta\left(1 \vee |\mathcal{R}_t|\right) A_i\alpha.
\end{aligned}$$

We apply this fact in Line (A.3), below.

$$\begin{aligned}
\text{FDR}(t) &= \mathbb{E}\left[\frac{\sum_{\{i \leq t : i \in \mathcal{H}_0\}} 1\left(i \in \mathcal{R}_t\right)}{1 \vee |\mathcal{R}_t|}\right] \\
&\leq \mathbb{E}\left[\frac{\sum_{\{i \leq t : i \in \mathcal{H}_0\}} 1\left(P_i \leq \beta(1 \vee |\mathcal{R}_t|)A_i\alpha\right)}{1 \vee |\mathcal{R}_t|}\right] &\text{(A.3)} \\
&= \sum_{\{i \leq t : i \in \mathcal{H}_0\}} \mathbb{E}\left[\frac{1\left(P_i \leq \beta(1 \vee |\mathcal{R}_t|)A_i\alpha\right)}{1 \vee |\mathcal{R}_t|}\right] \\
&= \sum_{\{i \leq t : i \in \mathcal{H}_0\}} \mathbb{E}_{\mathcal{P}_{\tau_i}} \mathbb{E}\left[\frac{1\left(P_i \leq \beta(1 \vee |\mathcal{R}_t|)A_i\alpha\right)}{1 \vee |\mathcal{R}_t|} |\mathcal{P}_{\tau_i}\right]. &\text{(A.4)}
\end{aligned}$$

Within the inner expectation, Assumption 1 tells us that $A_i$ is constant, and Assumption 2 tells us that $P_i$ is stochastically lower bounded by a uniform variable on [0,1] (i.e., it is super-uniform conditional on $\mathcal{P}_{\tau_i}$). Using these facts along with Assumption 3, we can apply Lemma 3.2-ii from Blanchard and Roquain (2008)

to see that the inner expectation is less than or equal to $A_i\alpha$.[1] Plugging this in and recalling that $A_i$ is a function of $\mathcal{P}_{\tau_i}$, we have

$$\text{FDR}(t) \leq \sum_{\{i\leq t\,:\,i\in\mathcal{H}_0\}} \mathbb{E}\left[A_i\alpha\right] = \alpha\mathbb{E}\left[\sum_{\{i\leq t\,:\,i\in\mathcal{H}_0\}} A_i\right] \leq \alpha,$$

where the last inequality follows from the definition of $A_i$.

As noted in Section 4.1, all of these steps remain unchanged if we replace $\mathcal{P}_{\tau_i}$ throughout with $\mathcal{P}_{\tau_i}^{\text{obs}}$. □

**Part 2**

*Proof.* The proof is almost identical to the proof of Part 1. There are only two minor differences.

First, to show Eq (A.2), we must now cite the fact that shape functions are nondecreasing. The second difference comes where we previously used Assumption 3 to apply Lemma 3.2-ii from Blanchard and Roquain (2008) in order to show that the inner expectation in Eq (A.4) is less than or equal to $A_i\alpha$. Now, we instead use the fact that $\beta$ is a shape function to apply Lemma 3.2-iii from Blanchard and Roquain (2008), which again shows that the inner expectation in Eq (A.4) is no more than $A_i\alpha$. □

# B Power comparison between TOAD & $\text{Batch}_{\text{BH}}^{\text{PRDS}}$

We start by reviewing the $\text{Batch}_{\text{BH}}^{\text{PRDS}}$ algorithm proposed in the appendix from Zrnic et al. (2020), and then move on to compare TOAD against $\text{Batch}_{\text{BH}}^{\text{PRDS}}$. As the name suggests, $\text{Batch}_{\text{BH}}^{\text{PRDS}}$ starts by breaking down the sequence of p-values into "batches." For each batch $b$, the authors apply BH to the $b^{th}$ batch at an alpha level of $\alpha^{(b)}$. Let $n^{(b)}$ denote the size of the $b^{th}$ batch, and let $R^{(b)}$ be the number of hypotheses rejected from batch $b$. Here, we use superscript notation to help distinguish between batch indices and test indices. Zrnic et al. define a $\text{Batch}_{\text{BH}}^{\text{PRDS}}$ procedure as any method of defining alpha levels $\{\alpha^{(b)}\}_{b=1}^{\infty}$ that satisfies

$$\sum_{s\leq b} \alpha^{(s)} \frac{n^{(s)}}{n^{(s)} + \sum_{r<s} R^{(r)}} \leq \alpha \tag{B.1}$$

for all batches $b$, where $\alpha$ is the desired FDR control level. Additionally, Zrnic et al. require each $\alpha^{(s)}$ to depend only on the p-values from the preceding batches.

In order to compare TOAD and $\text{Batch}_{\text{BH}}^{\text{PRDS}}$, we first need to translate the above "batch" notation into the more general notation of "deadlines." Given a sequence of p-values $P_1, P_2, \ldots$, let $g_1, g_2, \ldots$ be "group" or "batch" labels for each p-value. For example, if we observe two batches, each of size two, then $(g_1, g_2, g_3, g_4) = (1, 1, 2, 2)$. Again, we generally use subscript "stage indices" to refer to the indices of hypotheses and tests, and use superscript "batch indices" to denote batch numbers. We define each deadline parameter $d_i = \max\{i' : g_i = g_{i'}\}$ to be the (stage) index of the last test that is in the same batch as $P_i$.

If batch $b$ ends at stage $t$, then the following notational equivalencies can be made.

- $g_t = b$ is the batch label for stage $t$ (i.e., for the $t^{th}$ hypothesis);
- $\mathcal{C}_t = \{i \leq t : g_i = g_t\}$ is the set of stage indices in the $b^{th}$ batch; and
- $n^{(b)} = n^{(g_t)} = |\mathcal{C}_t|$ is the size of batch $b$.

Equipped with this notation, we can formally compare TOAD and $\text{Batch}_{\text{BH}}^{\text{PRDS}}$.

*Remark* B.1. *(Power comparison) Given a sequence of alpha levels $\{\alpha^{(b)}\}_{b=1}^{\infty}$ used by the $Batch_{BH}^{PRDS}$ method, if we set $\beta$ to be the identity function and set*

$$A_i = \frac{\alpha^{(g_i)}}{\alpha\left(n^{(g_i)} + \sum_{s<g_i} R^{(s)}\right)},$$

*for all $i$, then any hypothesis rejected by $Batch_{BH}^{PRDS}$ is also rejected by TOAD.*

[1] In applying this lemma, we set $V$, $U$, and $c$ in Blanchard and Roquain's notation equal to $(1 \vee R_j)$, $P_j$, and $A_j\alpha$ in our notation, respectively.

### Proof of Remark B.1

*Proof.* First, we note that this choice of $A_i$ still satisfies our requirement that $A_i$ is a function of the preceding p-values. We also note that, for any stage $t$ at which a batch ends, we have

$$\begin{aligned}\sum_{i=1}^{t} A_i &= \sum_{i=1}^{t} \frac{\alpha^{(g_i)}}{\alpha\left(n^{(g_i)} + \sum_{s<g_i} R^{(s)}\right)} \\ &= \sum_{b=1}^{g_t} n^{(b)} \frac{\alpha^{(b)}}{\alpha\left(n^{(b)} + \sum_{s<b} R^{(s)}\right)} \\ &= \frac{1}{\alpha} \sum_{b=1}^{g_t} \alpha^{(b)} \frac{n^{(b)}}{\left(n^{(b)} + \sum_{s<b} R^{(s)}\right)} \\ &\leq 1,\end{aligned}$$

where the last line comes from Eq (B.1).

Next, we write a more explicit version of the $\text{Batch}_{\text{BH}}^{\text{PRDS}}$ procedure that is closer in format to Algorithm 1.

*Algorithm* B.1. *(Alternative description $Batch_{BH}^{PRDS}$) Take as input an alpha level for the first batch, denoted by $\alpha^{(1)}$.*

*For each stage $t$:*

1. *Let $\mathcal{R}_t^{old}$ be the set of hypotheses rejected in previous batches.*
2. *If the current batch does not end at stage $t$ (i.e., if $t < d_t$): reject $\mathcal{R}_t = \mathcal{R}_t^{old}$.*
3. *If the current batch ends at stage $t$ (i.e., if $t = d_t$):*
   - (a) *Recall that $\mathcal{C}_t = \{i \leq t : g_i = g_t\}$ is the set of hypothesis indices in the same batch as $H_t$, so that $n^{(g_t)} = |\mathcal{C}_t|$.*
   - (b) *Let $P_{(j,t)}$ denote the $j^{th}$ highest p-value from the set $\{P_i\}_{i\in\mathcal{C}_t}$, that is, the $j^{th}$ highest p-value in the current batch.*
   - (c) *Set $\tilde{S}_t = \max\left\{j \leq |\mathcal{C}_t| : P_{(j,t)} \leq \frac{j}{|\mathcal{C}_t|}\alpha^{(g_t)}\right\}$.*
   - (d) *Reject $\mathcal{R}_t = \mathcal{R}_t^{old} \cup \{i \in \mathcal{C}_t : P_i \leq P_{(\tilde{S}_t,t)}\}$.*
   - (e) *Define the alpha level $\alpha^{(t+1)}$ to be used in the next batch, in accordance with Eq (B.1).*

Above, all we have done is changed the notation to define indices at the test level instead of the batch level, and plugged in the steps of the BH procedure.

For all tests $i$, let $W_i = P_i/A_i$. Let $W_{(j,t)}$ to be the $j^{th}$ highest value in the set $\{W_i\}_{i\in\mathcal{C}_t}$. Since $A_i$ is constant within a batch $\mathcal{C}_t$, we know that $W_i$ is proportional to $P_i$ among the indices $i \in \mathcal{C}_t$. Thus,

$W_{(j,t)} = P_{(j,t)}/A_t$. This leads to an equivalent definition of $\tilde{S}_t$:

$$\begin{aligned}
\tilde{S}_t &= \max\left\{j \le |\mathcal{C}_t| : P_{(j,t)} \le \frac{j}{|\mathcal{C}_t|}\alpha_t\right\} \\
&= \max\left\{j \le |\mathcal{C}_t| : P_{(j,t)}/A_t \le \frac{j\alpha_t}{|\mathcal{C}_t|}A_t^{-1}\right\} \\
&= \max\left\{j \le |\mathcal{C}_t| : W_{(j,t)} \le \frac{j\alpha^{(g_t)}}{|\mathcal{C}_t|} \times \frac{\alpha\left(n^{(g_t)} + \sum_{s<g_t} R^{(s)}\right)}{\alpha^{(g_t)}}\right\} \\
&= \max\left\{j \le |\mathcal{C}_t| : W_{(j,t)} \le \frac{j\alpha}{|\mathcal{C}_t|}\left(n^{(g_t)} + \sum_{s<g_t} R^{(s)}\right)\right\} \\
&= \max\left\{j \le |\mathcal{C}_t| : W_{(j,t)} \le \frac{j\alpha}{|\mathcal{C}_t|}\left(|\mathcal{C}_t| + |\mathcal{R}_t^{\text{old}}|\right)\right\} \\
&= \max\left\{j \le |\mathcal{C}_t| : W_{(j,t)} \le \alpha\left(j + \frac{j}{|\mathcal{C}_t|} \times |\mathcal{R}_t^{\text{old}}|\right)\right\}.
\end{aligned}$$

Thus, Step 3d is equivalent to rejecting $\mathcal{R}_t^{\text{old}} \cup \{i \in \mathcal{C}_t : W_i \le W_{(\tilde{S}_t,t)}\}$. All that remains is to show that $\tilde{S}_t \le S_t$, where $S_t$ is the value in Eq (3). This follows immediately from the fact that $j/|\mathcal{C}_t| \le 1$. □

# C Sufficient conditions for Assumption 3

First, we review the definition of positive regression dependence on a subset (PRDS; Benjamini and Yekutieli, 2001). Given a value $t \in \mathbb{N}$, let $\mathbf{P} = (P_1, \dots, P_t)$ (we suppress the dependence on $t$ for brevity). We say that a set of $k$-dimensional vectors $D \in [0,1]^k$ is *increasing* if, for any vector $\mathbf{x} = (x_1, \dots, x_t) \in D$ and any vector $\mathbf{y} = (y_1, \dots, y_t)$ satisfying $x_i \le y_i$ for all $i$, it must also be that $\mathbf{y} \in D$. Given a subset $I_0 \subseteq \{1, \dots t\}$, the PRDS condition states that, for any increasing set $D$ and any $j \in I_0$, the conditional probability $\mathbb{P}(\mathbf{P} \in D | P_j = u)$ is nondecreasing in $u$.

Following the argument of Blanchard and Roquain (2008; see Proposition 3.6 and citations therein), we outline two sufficient conditions that imply Assumption 3.

*Condition* C.1. *For any $t \in \mathbb{N}$, increasing any of the first $t$ p-values cannot increase the total number of discoveries produced by time $t$.*

*Condition* C.2. *For any $j, t \in \mathbb{N}$ such that $j \le t$ and $H_j \in \mathcal{H}_0$, and for any increasing set $D \in [0,1]^t$, the conditional probability $\mathbb{P}(\mathbf{P} \in D | P_j = u, \mathcal{P}_{\tau_j})$ is nondecreasing in $u$.*

Condition C.1 holds, for example, if all parameters $A_i$ are prespecified, or if they are monotonically decreasing in the p-values observed so far. Alternatively, Condition C.1 holds if we set $A_1, A_2, \dots$ equal to a predetermined sequence of constants $a_1, a_2, \dots$ until a certain number of discoveries are found, and set $A_t = 0$ afterwards. Condition C.2 is a modified version of the PRDS requirement.

*Remark* C.1. *If Conditions C.1 & C.2 hold then Assumption 3 holds.*

### Proof of Remark C.1

*Proof.* (Adapted from Blanchard and Roquain, 2008) For any $0 \le r \le t$, let $D_r \subseteq [0,1]^t$ be the set of all possible p-values that produce no more than $1 \vee r$ discoveries by stage $t$. Since increasing any p-value will not increase the number of discoveries by stage $t$, we know that $D_r$ is an increasing set. For any $u < u'$, let

$\gamma = P(P_j \leq u | P_j \leq u', \mathcal{P}_{\tau_j})$. Then

$$
\begin{aligned}
&\mathbb{P}(1 \vee |\mathcal{R}_t| \leq r | P_j \leq u', \mathcal{P}_{\tau_j}) \\
&= \mathbb{P}(\mathbf{P} \in D_r | P_j \leq u', \mathcal{P}_{\tau_j}) && \text{(C.1)} \\
&= \mathbb{E}\left[\mathbb{P}(\mathbf{P} \in D_r | P_j, \mathcal{P}_{\tau_j}) \quad | \quad P_j \leq u', \mathcal{P}_{\tau_j}\right] \\
&= \quad \mathbb{E}\left[\mathbb{P}(\mathbf{P} \in D_r | P_j, \mathcal{P}_{\tau_j}) \quad | \quad P_j \leq u, \mathcal{P}_{\tau_j}\right] \gamma && \text{(C.2)} \\
&\quad + \mathbb{E}\left[\mathbb{P}(\mathbf{P} \in D_r | P_j, \mathcal{P}_{\tau_j}) \quad | \quad u < P_j \leq u', \mathcal{P}_{\tau_j}\right] (1-\gamma). && \text{(C.3)}
\end{aligned}
$$

Under Condition C.2, the expectation in Line (C.2) is smaller than the expectation in Line (C.3). Thus, if we were to replace the expectation in Line (C.3) with the expectation in Line (C.2), the sum shown in Lines (C.2)-(C.3) would be reduced. Making this substitution and combining terms gives

$$
\begin{aligned}
\mathbb{P}(1 \vee |\mathcal{R}_t| \leq r | P_j \leq u', \mathcal{P}_{\tau_j}) &\geq \mathbb{E}\left[\mathbb{P}(\mathbf{P} \in D_r | P_j, \mathcal{P}_{\tau_j}) \quad | \quad P_j \leq u, \mathcal{P}_{\tau_j}\right] \\
&= \mathbb{P}(\mathbf{P} \in D_r | P_j \leq u, \mathcal{P}_{\tau_j}) \\
&= \mathbb{P}(1 \vee |\mathcal{R}_t| \leq r | P_j \leq u, \mathcal{P}_{\tau_j}).
\end{aligned}
$$

This proves the result. □

# D FDR for Naive-BH

Here, we show that Naive-BH controls the FDR whenever the p-values are PRDS (see Appendix C; and Benjamini and Yekutieli, 2001) on the subset of test statistics corresponding to the true null hypotheses.

Let $R^{(b)}$ be the number of rejections from the $b^{th}$ batch and let $V^{(b)}$ denote the number of erroneous rejections from the $b^{th}$ batch. Note that $\lfloor t/n_{\text{batch}} \rfloor$ is the number of batches that have completed by stage $t$. Recall also that Naive-BH uses an alpha level of $\alpha(t_{\max}/n_{\text{batch}})^{-1}$ for each batch. We have

$$
\begin{aligned}
FDR(t) = \mathbb{E}\left[\frac{\sum_{\{b \leq \lfloor t/n_{\text{batch}} \rfloor\}} V^{(b)}}{\sum_{\{b' \leq \lfloor t/n_{\text{batch}} \rfloor\}} R^{(b')}}\right] &= \sum_{\{b \leq \lfloor t/n_{\text{batch}} \rfloor\}} \mathbb{E}\left[\frac{V^{(b)}}{\sum_{\{b' \leq \lfloor t/n_{\text{batch}} \rfloor\}} R^{(b')}}\right] \\
&\leq \sum_{\{b \leq \lfloor t/n_{\text{batch}} \rfloor\}} \mathbb{E}\left[\frac{V^{(b)}}{R^{(b)}}\right] \\
&\leq \sum_{\{b \leq \lfloor t/n_{\text{batch}} \rfloor\}} \alpha \frac{n_{\text{batch}}}{t_{\max}} && \text{(D.1)} \\
&\leq \frac{t_{\max}}{n_{\text{batch}}} \times \alpha \frac{n_{\text{batch}}}{t_{\max}} \\
&= \alpha,
\end{aligned}
$$

where Line (D.1) comes from the well-known result that BH controls the (within batch) FDR under the PRDS assumption (Theorem 1.2 from Benjamini and Yekutieli, 2001).

# E Additional Simulations

As a second set of simulations, we consider the setting described by Zrnic et al. (2020) and Javanmard and Montanari (2018) in which the amount of signal can vary drastically across test statistics. For each index $i$ associated with an alternative distribution, we draw $\mu_i$ from a random normal distribution with mean zero and variance $2\log(t_{\max}) \approx 16$. Here, we set $P_i = 2\Phi(-|Z_i|)$ to be the p-value resulting from a two-sided test of $H_i$.

Figures E.1 & E.2 show the results of these simulations. Overall, the pattern resembles what we observe in our main simulations. Here however, both the differences in power and the degree of FDR inflation are less pronounced.

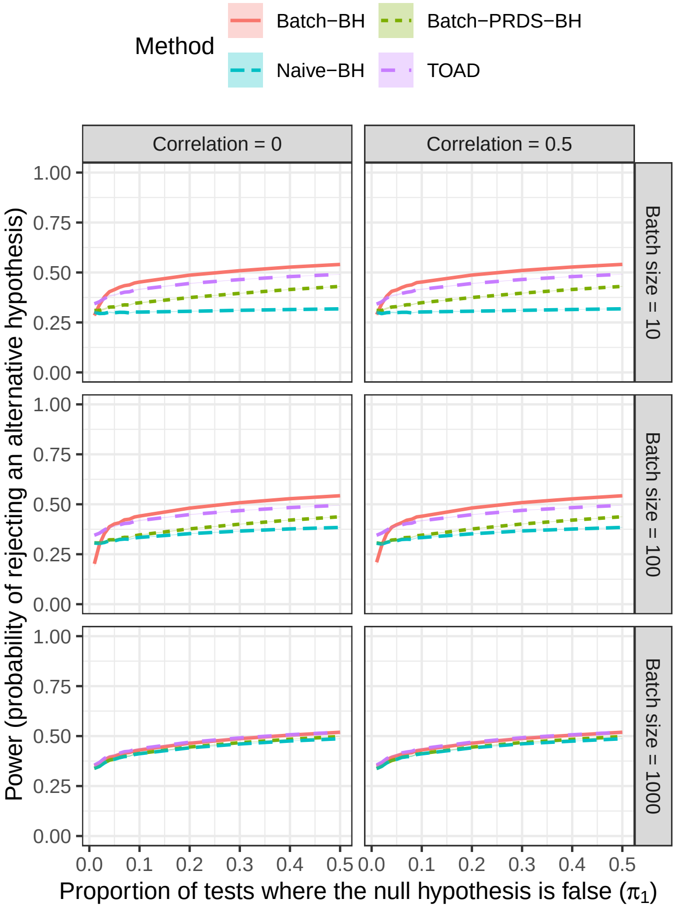


Figure E.1: Simulated power under randomly selected values for the mean parameters

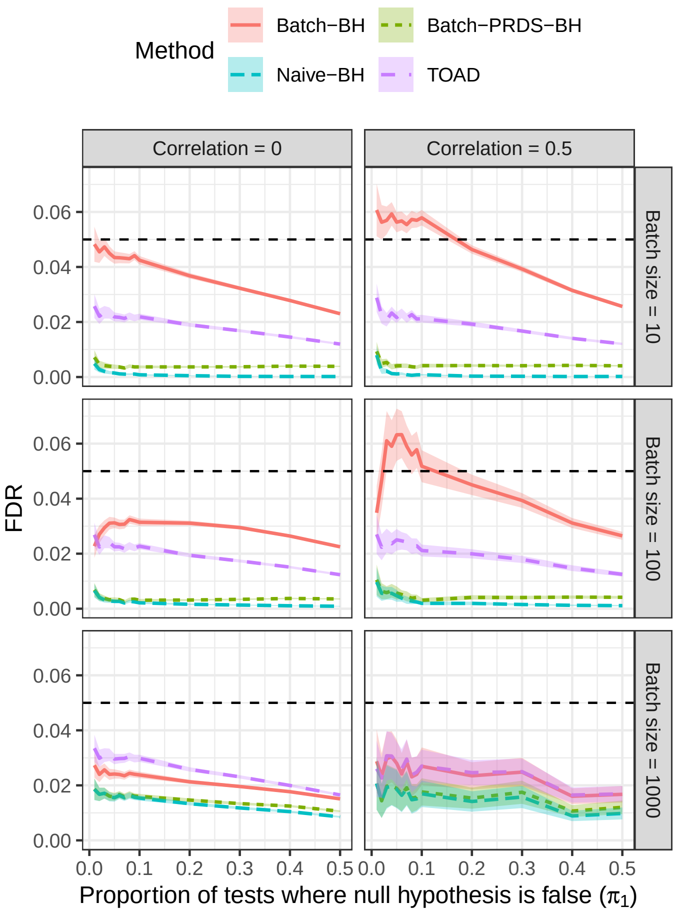


Figure E.2: Simulated FDR under randomly selected values for the mean parameters

# F Forgetting Antiquated Tests

*Proof.* Here, we show that Theorem 1 still holds if we replace $\mathrm{FDR}(t)$ with $\mathrm{FDR}_{\mathrm{recent}}(t)$; replace $\mathcal{R}_t^{\mathrm{old}}$ with the empty set $\emptyset$ throughout the procedure; and relax the requirement that $\sum_{i=1}^{\infty} A_i \leq 1$ to instead require that $\sum_{i\in\mathcal{C}_t} A_i \leq 1$ for all $t$.

To show Part 1, suppose the $H_i$ is rejected at stage $t$. We know that

$$P_i/A_i = W_i \leq W_{(S_t,t)} \leq \alpha\beta\left(S_t\right) = \alpha\beta\left(|\mathcal{R}_t|\right) \leq \alpha\beta\left(1 \vee |\mathcal{R}_t|\right).$$

Thus, rejecting any hypothesis $H_i$ at time $t$ requires that

$$P_i \leq \beta\left(1 \vee |\mathcal{R}_t|\right) A_i\alpha.$$

We applying this fact, we have

$$\begin{aligned} \mathrm{FDR}_{\mathrm{recent}}(t) &= \mathbb{E}\left[\frac{\sum_{\{i\leq t\,:\,i\in\mathcal{H}_0\cap\mathcal{C}_t\}} 1\left(i \in \mathcal{R}_t\right)}{1 \vee |\mathcal{R}_t \cap \mathcal{C}_t|}\right] \\ &\leq \sum_{\{i\leq t\,:\,i\in\mathcal{H}_0\cap\mathcal{C}_t\}} \mathbb{E}_{\mathcal{P}_{\tau_i}} \mathbb{E}\left[\frac{1\left(P_i \leq \beta(1\vee R_t)A_i\alpha\right)}{1 \vee |\mathcal{R}_t \cap \mathcal{C}_t|} |\mathcal{P}_{\tau_i}\right]. \end{aligned} \tag{F.1}$$

As in Appendix A.2, we apply Lemma 3.2-ii from Blanchard and Roquain (2008) to see that the inner expectation is no more than $A_i\alpha$. Thus,

$$\mathrm{FDR}_{\mathrm{recent}}(t) \leq \sum_{\{i\leq t\,:\,i\in\mathcal{H}_0\cap\mathcal{C}_t\}} \mathbb{E}\left[A_i\alpha\right] = \alpha\mathbb{E}\left[\sum_{\{i\leq t\,:\,i\in\mathcal{H}_0\cap\mathcal{C}_t\}} A_i\right] \leq \alpha.$$

To show Part 2, we follow the same steps with the exception of applying Lemma 3.2-iii from Blanchard and Roquain (2008) to Eq (F.1). □

# References


Benjamini, Y. and Yekutieli, D. (2001). The control of the false discovery rate in multiple testing under dependency. *Ann. Stat.*, 29(4):1165–1188.

Blanchard, G. and Roquain, E. (2008). Two simple sufficient conditions for FDR control. *EJSS*, 2(none):963–992.

Javanmard, A. and Montanari, A. (2018). Online rules for control of false discovery rate and false discovery exceedance. *aos*, 46(2):526–554.

Zrnic, T., Jiang, D., Ramdas, A., and Jordan, M. (2020). The power of batching in multiple hypothesis testing. In Chiappa, S. and Calandra, R., editors, *Proceedings of the Twenty Third International Conference on Artificial Intelligence and Statistics*, volume 108 of *Proceedings of Machine Learning Research*, pages 3806–3815. PMLR.
